# Supplementary material for: Aberration-Aware Depth-from-Focus
Source: arXiv:2303.04654 source file (2023-07-17)
Supplement: Supplementary file 5 [file fig.tex]

\begin{figure*}[!ht]
    \centering
    \setlength{\tabcolsep}{1pt}
    \resizebox{\textwidth}{!}{
    \begin{tabular}{ccc}
         \includegraphics[width=3cm]{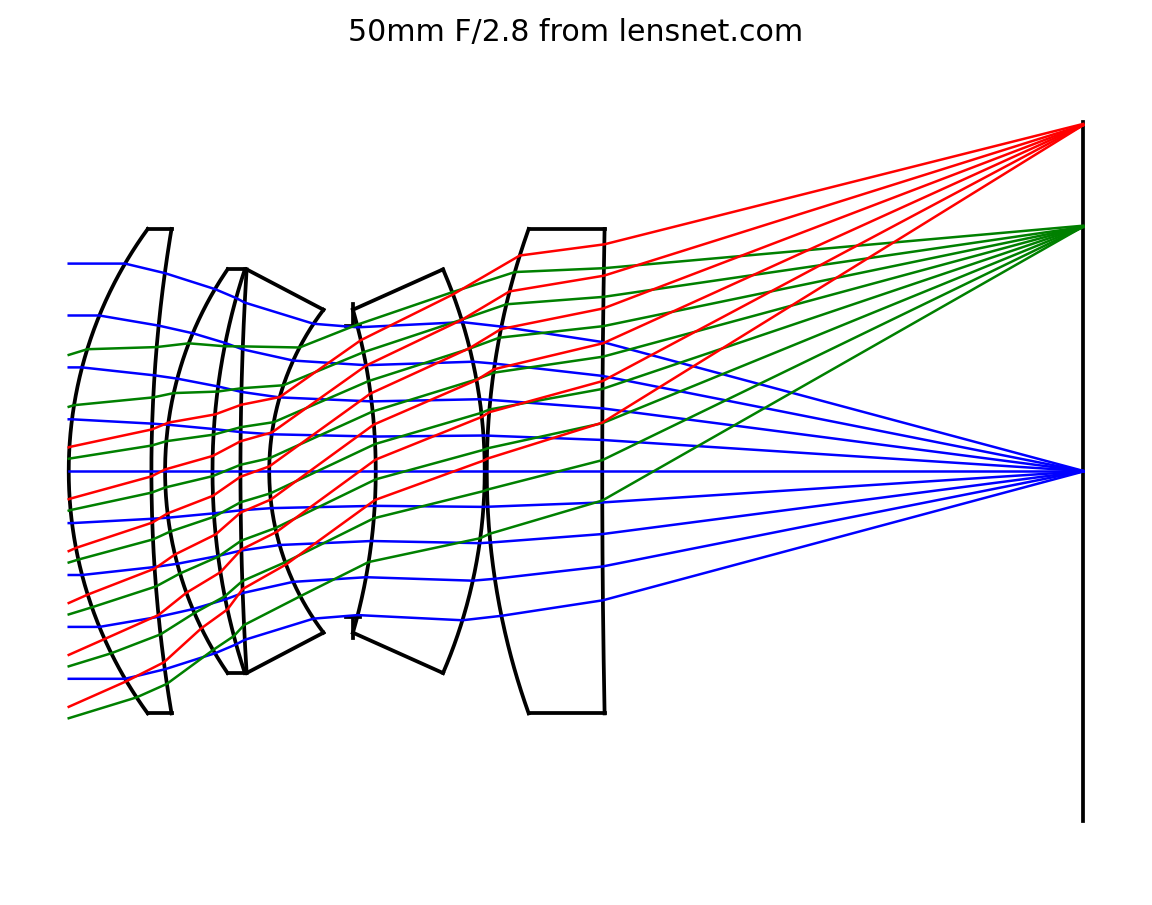}
         &
         \includegraphics[width=3cm]{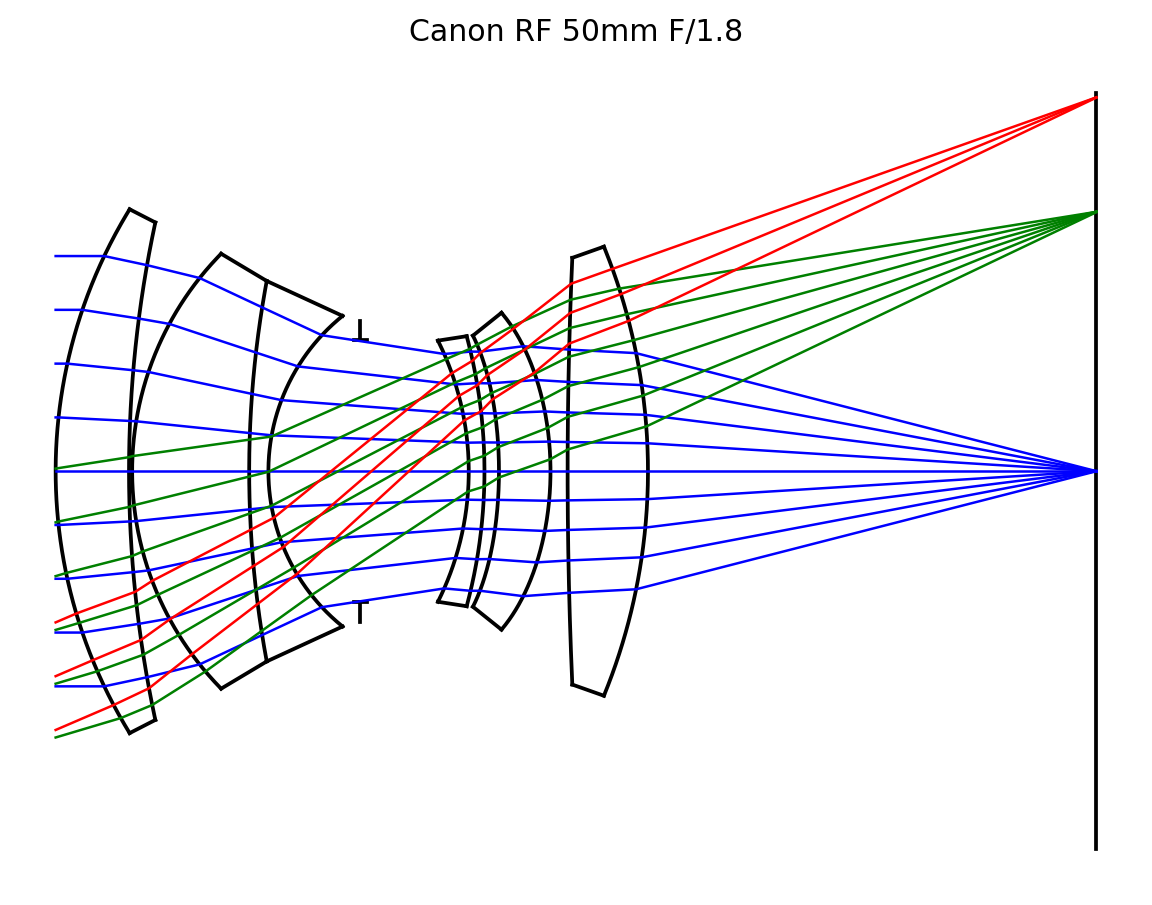}
    \end{tabular}
    }
    \caption{Lens setup. Left: a 50mm F/2.8 lens from \href{http://lensnet.herokuapp.com/}{lensnet.com}~\cite{cote2021deep}. Right: the Canon RF 50mm F/1.8 lens.}
    \label{fig:lens}
\end{figure*}
