# Supplementary material for: Aberration-Aware Depth-from-Focus
Source: arXiv:2303.04654 source file (2023-07-17)
Supplement: Supplementary file 7 [file fig.tex]

\begin{figure*}[!ht]
    \centering
    \setlength{\tabcolsep}{1pt}
    \resizebox{0.8\textwidth}{!}{
    \begin{tabular}{cc}
         \includegraphics[width=0.45\textwidth]{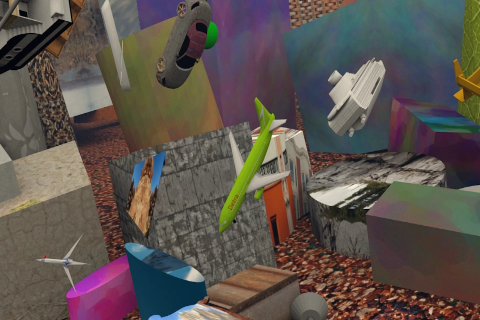}
         &
         \includegraphics[width=0.45\textwidth]{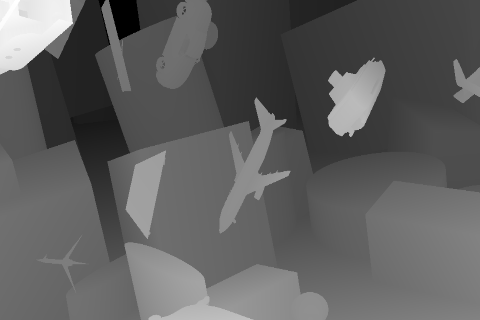}
         \\
         (a) All-in-focus RGB image
         &
         (b) Ground-truth depth map
         \\
         \includegraphics[width=0.45\textwidth]{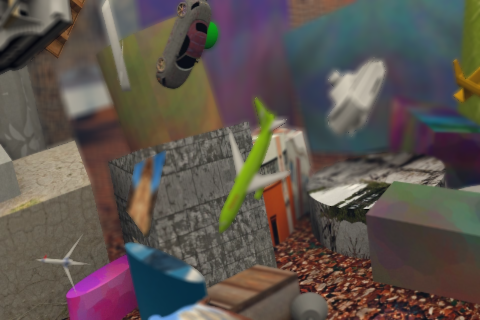}
         &
         \includegraphics[width=0.45\textwidth]{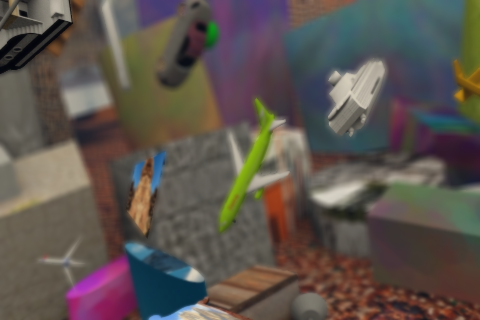}
         \\
         (c) Focused image example 1
         &
         (d) Focused image example 2
    \end{tabular}
    }
    \caption{Simulated focal stacks with RGBD images.}
    \label{fig_supp:simulated}
\end{figure*}
